# Supplementary material for: Atomic monolayer deposition on the surface of nanotube mechanical resonators
Source: arXiv:1404.5833 source file (2014-04-24)
Supplement: Supplementary file 1 [file Supplementary_Material.pdf]

# Supplementary material for: Atomic monolayer deposition on the surface of nanotube mechanical resonators

A. Tavernarakis,<sup>1</sup> J. Chaste,<sup>2,\*</sup> A. Eichler,<sup>1,2,†</sup> G. Ceballos,<sup>2</sup> M. C. Gordillo,<sup>3</sup> J. Boronat,<sup>4</sup> and A. Bachtold<sup>1,2</sup>

<sup>1</sup>*ICFO - Institut de Ciències Fotoniques, Mediterranean Technology Park, 08860 Castelldefels, Barcelona, Spain*

<sup>2</sup>*Institut Català de Nanotecnologia, Campus de la UAB, E-08193 Bellaterra, Spain*

<sup>3</sup>*Departamento de Sistemas Físicos, Químicos y Naturales,  
Universidad Pablo de Olavide, Carretera de Utrera, km 1, E-41013 Sevilla, Spain*

<sup>4</sup>*Departament de Física i Enginyeria Nuclear, Universitat Politècnica  
de Catalunya, B4-B5 Campus Nord, 08034 Barcelona, Spain*

## I. NANOFABRICATION PROCESS

The nanofabrication process goes as follows. First, a trench is etched into a highly resistive Si wafer coated with  $\text{SiO}_2$  and  $\text{Si}_3\text{N}_4$ . W and Pt are evaporated into the trench to create a gate electrode (G). In a second lithography step, a continuous line is exposed across the trench with the electron beam. After a deposition of W/Pt and lift-off, the line results in the source (S) and (D) electrodes separated by the trench. W/Pt are chosen because of their high melting points. An island of catalyst is then patterned on the source/drain electrodes using electron-beam lithography. A chemical vapour deposition furnace (Lindberg Blue M TF55035C) is used to grow nanotubes at  $800^\circ\text{C}$ . Since the growth is the last step of the fabrication process, we avoid contamination on the nanotube caused by the nanofabrication process.

## II. EXPERIMENTAL SETUP

The experimental setup consists of a home-built, ultra-high vacuum (UHV) chamber. A vacuum of  $\sim 3 \cdot 10^{-11}$  mbar can be reached after a two-day bake-out at  $110^\circ\text{C}$ . The sample is attached to the cold finger of a liquid helium insert (Janis, ST-400). The temperature of the sample can be varied from 4 to 300 K with a temperature controller (LakeShore 332). The sample is glued onto a printed circuit board, which is electrically connected to radio-frequency, UHV-compatible cables. Gas atoms are dosed into the UHV chamber with a pinhole microdoser.

## III. CHARACTERIZATION OF THE NANOTUBE RESONATOR

We select nanotubes that are metallic with a small energy gap in order to be able to grow monolayers of noble gas atoms that are commensurate with the carbon surface. This selection is done by measuring the conductance  $G$

---

\*Present address: CNRS, Laboratoire de Photonique et de Nanostructures, UPR20, route de Nozay, 91460 Marcoussis, France

†Present address: Department of Physics, ETH Zurich, Schafmattstrasse 16, 8093 Zurich, Switzerland.

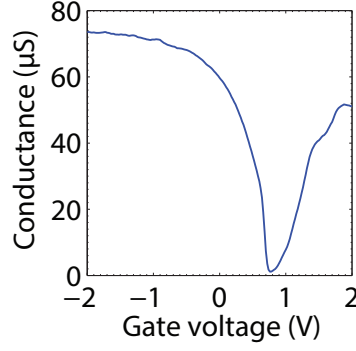

FIG. S1: The nanotube conductance as a function of gate voltage prior to current annealing. The temperature is 65 K. After current annealing, the gap shifts to zero gate voltage.

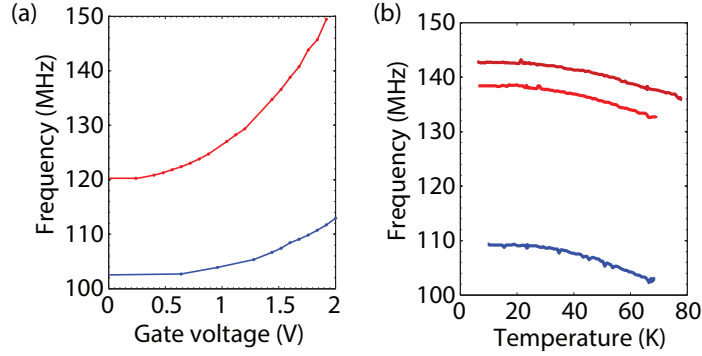

FIG. S2: (a) The resonance frequencies of the first two eigenmodes as a function of gate voltage measured at 65 K after current annealing. (b) Resonance frequencies as a function of temperature measured at different gate voltages.

as a function of the voltage  $V_g$  applied to the gate electrode [1]. Figure (S1) shows the  $G - V_g$  characteristic of the nanotube resonator discussed in the Letter.

The vibrations of the nanotube resonator are driven and detected electrically using the frequency modulation (FM) mixing technique [2]. We apply a frequency modulated oscillating voltage with amplitude  $V_{\text{FM}} \simeq 1$  mV on the source electrode. The resulting mixing current  $I_{\text{mix}}$  (at typically 671 Hz) is detected at the drain electrode using a lock-in amplifier. This current is largest at the resonance frequency.

The mechanical eigenmodes are characterized by measuring the resonance frequency  $f^0$  as a function of gate voltage (Fig. S2(a)). The lowest-frequency eigenmode detected in Fig. S2(a) corresponds to the lowest-energy mode vibrating (essentially) parallel to the surface of the gate electrode, whereas the second eigenmode in Fig. S2(a) is assigned to the lowest-energy mode vibrating in a direction (essentially) perpendicular to the gate electrode, as shown in Ref. [3]. Mass sensing measurements in the Letter are carried out with the second mode, because  $I_{\text{mix}}$  is larger. As depicted in Fig. S2(b), the resonance frequencies increase upon lowering temperature. This behaviour is attributed to the thermal expansion of the electrodes which modifies the spring constant of the nanotube resonator [4]. However, the ratio between the resonance frequencies measured at different  $V_g$  remains constant upon varying temperature (the largest deviation is less than 1 %). In other words, the ratio between the spring constants at different  $V_g$  is independent of temperature. This is important for converting  $f^0$  into coverage as we will see in the next section.

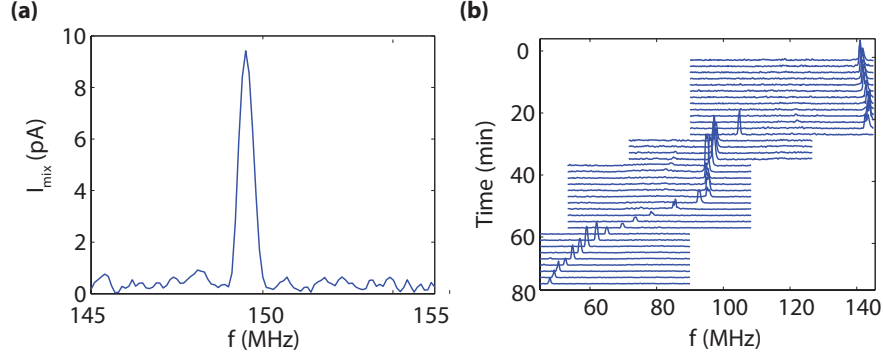

FIG. S3: (a) Resonance of the mixing current  $I_{\text{mix}}$ . (b) Raw data showing consecutive resonances in  $I_{\text{mix}}$  upon lowering temperature while dosing Kr atoms.

The adsorption of noble gas atoms onto the nanotube is monitored by measuring the resonance frequency. For this, we continuously record the response of the nanotube to the driving frequency. Figure S3(a) shows the resonance of  $I_{\text{mix}}$  as a function of the driving frequency. In practice, when we lower the temperature while dosing noble gas atoms, the scan range of the driving frequency has to be adjusted manually in order to keep track of  $f^0$  (see Fig. S3(b)). One frequency scan takes typically one minute. The height of the resonance in  $I_{\text{mix}}$  varies upon decreasing  $T$  because of the variation of the transconductance of the nanotube. The quality factor and the associated linewidth are not important for such adsorption experiments, since the shift of the resonance frequency  $f^0$  induced by the adsorption of noble gas atoms is large. The quality factor of the nanotube resonator discussed in the Letter is modest. It is of the order of 100.

#### IV. CONVERTING RESONANCE FREQUENCY INTO COVERAGE

We assume that adsorbed atoms are homogeneously distributed along the nanotube, and the spring tension is insensitive to the tension induced by the interaction between noble gas atoms (which is two orders of magnitude weaker than that of covalent C-C bonds). The resonance frequency of the pristine tube (that is, when not dosing atoms) is  $f_{\text{prist}}^0 = 1/2\pi \cdot (k_{\text{prist}}/m_{\text{NT}})^{1/2}$ . The resonance frequency when dosing atoms for adsorption is  $f_{\text{ads}}^0 = 1/2\pi \cdot (k_{\text{ads}}/m_{\text{NT}} + \Delta m)^{1/2}$ . Here,  $m_{\text{NT}}$  is the mass of the nanotube and  $\Delta m$  is the mass of the adsorbed atoms. The spring constants  $k_{\text{prist}}$  and  $k_{\text{ads}}$  are functions of  $T$  and  $V_g$ , but we know from the last section that  $A \equiv k_{\text{ads}}/k_{\text{prist}}$  is independent of temperature provided that, for each measurement  $f_{\text{prist}}^0(T)$  and  $f_{\text{ads}}^0(T)$ , the gate voltage is kept constant. The coverage  $\varphi$  is defined as the ratio between the number of adsorbed atoms  $N_{\text{ads}} = \Delta m/m_{\text{ads}}$  and the number of carbon atoms of the nanotube  $N_{\text{C}} = m_{\text{NT}}/m_{\text{C}}$  where  $m_{\text{C}}$  and  $m_{\text{ads}}$  are the atomic masses of carbon and adsorbed atoms, respectively. Simple algebra leads to

$$\varphi(T) = \frac{m_{\text{C}}}{m_{\text{ads}}} \left[ A \cdot \left( \frac{f_{\text{prist}}^0(T)}{f_{\text{ads}}^0(T)} \right)^2 - 1 \right]. \quad (1)$$

The constant  $A$  is fixed so that  $\varphi = 0$  at temperatures much larger than  $T_c$  (when impinging atoms depart very rapidly from the nanotube, so that  $N_{\text{ads}}$  remains close to zero).

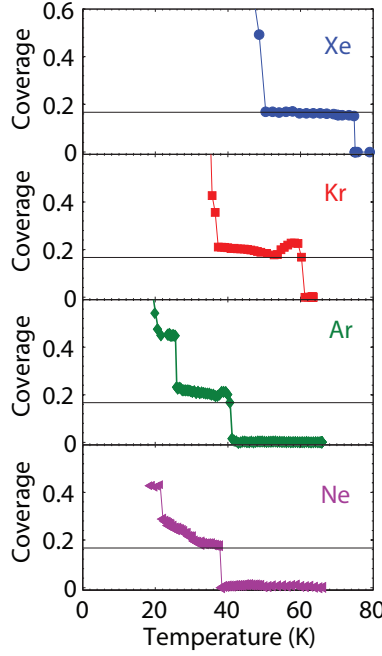

FIG. S4: Coverage upon increasing temperature. The vacuum is in the  $10^{-11}$  mbar range. The noble gas atoms are dosed onto the nanotube at 4 K prior to these measurements.

## V. EVAPORATING MONOLAYERS FROM THE NANOTUBE

In the Letter, we describe measurements monitoring the growth of noble gas atom monolayers onto the nanotube. Here, we present data where we evaporate the monolayers from the nanotube by heating the cryostat from low  $T$  when not dosing atoms (Fig. S4). The  $T$  ramping rate is 0.03 K/s. The vacuum is in the  $10^{-11}$  mbar range. The coverage jumps from  $\sim 1/6$  to 0 at a temperature that is up to 10 K higher than  $T_c$  in Fig. 3 of the Letter.

In Fig. S4, the measurement with Xe features a clear plateau at  $\varphi = 1/6$  over a large temperature range. By contrast, the plateau is much less robust for Kr. In particular, the coverage increases significantly above  $1/6$  close to the temperature at which  $\varphi$  jumps to zero. A similar behavior, albeit less pronounced, is observed for Ar. This increase in  $\varphi$  might be attributed to the rearrangement of the atoms on the nanotube surface, facilitated by thermal energy, and the supply of additional atoms from *e.g.* the metal electrodes. More work is needed to understand this behavior.

## VI. TIME DEPENDENCE OF THE GROWTH OF MONOLAYERS

In Fig. S5 we monitor the coverage as a function of time at a constant temperature (50 K) upon dosing Xe atoms at two different pressures  $P$  ( $8 \cdot 10^{-8}$  and  $3 \cdot 10^{-7}$  mbar). Once the coverage reaches  $\sim 1/6$ , it stops increasing. The time to reach  $\sim 1/6$  is faster when the pressure is higher.

The flux of atoms impinging the nanotube is given by  $I_{NT} = P/(2\pi m_{Xe} kT)^{1/2}$ . We assume that the cross section of the nanotube is  $d_{NT} L_{NT}$  where  $d_{NT}$  is the nanotube diameter and  $L_{NT}$  is the nanotube length. The number of carbon atoms of the nanotube is  $2\pi d_{NT} L_{NT}/S_G$  where  $S_G = 5.2 \cdot 10^{-20}$  m<sup>2</sup> is the surface of the graphite hexagon.

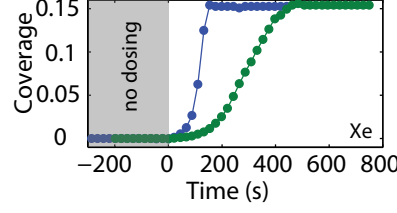

FIG. S5: Coverage as a function of time at 50 K upon dosing Xe atoms at two different pressures ( $8 \cdot 10^{-8}$  and  $3 \cdot 10^{-7}$  mbar for green and blue circles, respectively).

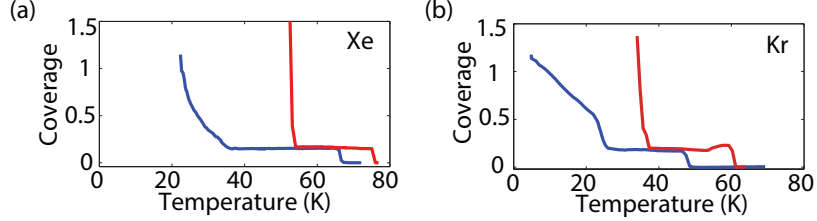

FIG. S6: Coverage of Xe and Kr upon lowering temperature (blue curve) and increasing temperature (red curve). The pressure is  $3 \cdot 10^{-7}$  mbar for the blue curves, whereas it is  $\sim 3 \cdot 10^{-11}$  mbar for the red curves. The  $T$  ramping rate is 0.016 K/s and 0.03 K/s for the blue and red curves, respectively.

As a result, the growth time to reach  $\varphi = 1/6$  is

$$t_{1/6} = \frac{2\pi(2\pi m_{\text{Xe}} k_B T)^{1/2}}{6S_G P}. \quad (2)$$

Since the atoms are supplied from a reservoir at 300 K, we expect that the growth time is  $t_{1/6} = 50$  s for  $P = 3 \cdot 10^{-7}$  mbar, which is consistent with the measurements.

## VII. MULTILAYER FORMATION

Figure S6 depicts the coverage upon lowering the temperature while dosing Xe and Kr atoms (blue curves) as well as the coverage of layers of Xe and Kr upon increasing the temperature without dosing gas atoms. Above  $\varphi = 1/6$  the dependance is monotonic without any plateaus even when the coverage gets larger than one.

## VIII. ADDITIONAL DEVICE

Figure (S7) shows the growth of monolayers of Xe and Ne onto another nanotube resonator. The characteristic temperatures  $T_c$  are similar to those measured with the first nanotube. Below  $T_c$  the coverage of Xe remains constant at  $\varphi \simeq 1/6$  over a large temperature range, while the coverage of Ne continuously increases upon lowering temperature. Note that a second plateau in coverage appears in the measurements with Xe. This second plateau might be attributed to the formation of a second layer.

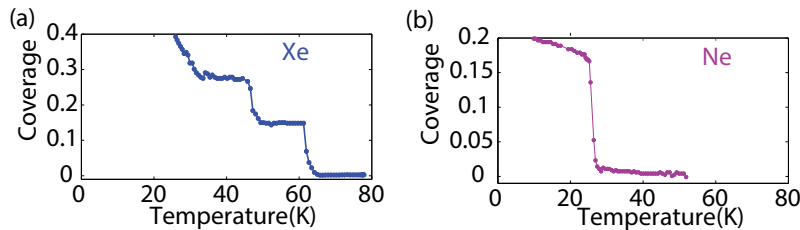

FIG. S7: Coverage upon lowering temperature measured on another nanotube resonator while dosing Xe and Ne atoms. The pressure is  $2 \cdot 10^{-7}$  mbar and the T ramping rate is 0.016 K/s for all measurements.

## IX. THEORETICAL CALCULATIONS

In a first type of simulations, we calculated the ground state phase of the noble gases under study adsorbed on the outer surface of different isolated carbon nanotubes in the limit of zero temperature. Since all the adsorbates considered in this work are relatively heavy atoms, we neglected the influence of their respective zero-point kinetic energies and followed a potential-energy minimization scheme, exact only at  $T = 0$ . To do so, we placed a set of  $m$  noble gas atoms on a circumference whose plane was perpendicular to the main axis ( $z$ ) of the tube ( $m \geq 9$ , with an upper limit that depended on the diameter of the tube). We denoted the radius of that circumference by  $R$ . Another atom circle was located parallel to the first one but separated from it by a given distance,  $d$ , in the  $z$  direction. The position of this second set of atoms was rotated by an angle of  $\pi/m$  with respect to the initial set. Those  $2m$  atoms form a unit cell of length  $2d$  which was repeated ten times to produce a periodic solid structure. Underneath, those regularly disposed atoms, we generated the corresponding carbon nanotube. We considered mainly armchair nanotubes of the type  $(n, n)$  but we checked that our results were qualitatively the same for zigzag,  $(n, 0)$ , nanotubes of similar diameters ( $n$  being the nanotube index in the standard nomenclature). We modeled the interaction between carbon and gas atoms by anisotropic Lennard-Jones potentials and the interaction between gas atoms by isotropic Lennard-Jones potentials, with parameters taken from Refs. [5] for Ne, [6] for Ar, [7] for Kr, and [8] for Xe. For a fixed  $m$ , we varied  $d$  and  $R$  to find the minimum energy per gas atom  $E$ , and the corresponding coverage. If different  $m$  rendered energy minimum at the same coverage, we would consider only the structure with the lowest  $E$ .

In a second type of simulations, we performed the calculations of the same system described above but at finite temperature  $T$ . We studied the adsorption of the noble gases using Metropolis Monte Carlo, in which configurations are generated according to the Boltzmann probability density law,  $\exp[-\beta V(\mathbf{R})]$ , with  $\beta = 1/T$  and  $V(\mathbf{R})$  the potential felt by gas atoms. The aim of this approach was to analyze the stability of crystal phases in the range of temperature and coverage measured in the experiments.

Figure S8(a) shows the energy per gas atom as a function of coverage for Xe in the limit of zero temperature. We see two minima, one at a coverage of  $\sim 1/6$  and one in the coverage range 0.185 – 0.195. The  $1/6$  coverage corresponds to a structure of a commensurate  $\sqrt{3} \times \sqrt{3}$  solid wrapped around the nanotube. The coverage in the 0.185 – 0.195 range corresponds to an incommensurate crystal. The energy is lowest at the coverage  $1/6$  for (24,24) and (28,28) nanotubes. Carrying out the second type of simulations, we found that these commensurate crystals are stable up to  $\sim 80$  K.

Figure S8(b) shows the energy as a function of coverage for Ne (blue) and Ar (red) in the limit of zero temperature.

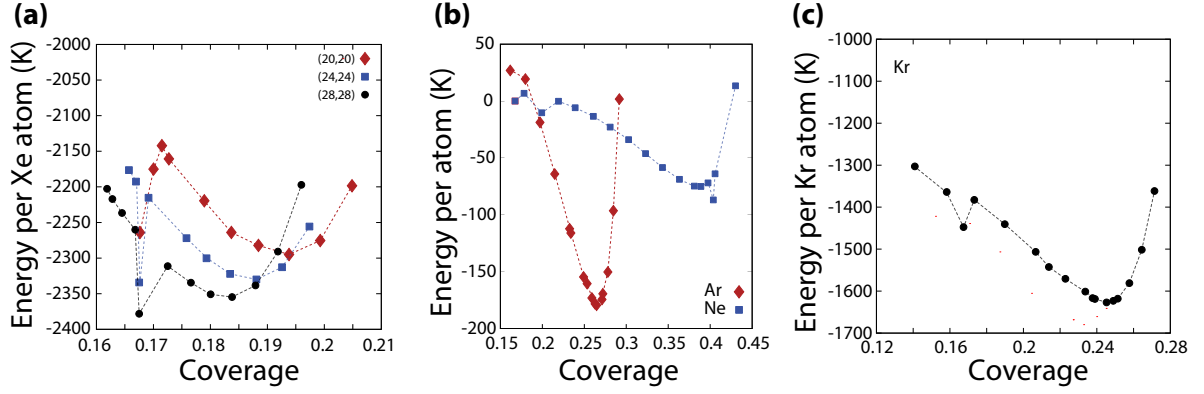

FIG. S8: (a) Energy per Xe atom as a function of the coverage for three  $(n,n)$  carbon nanotubes. (b) Energy per atom as a function of the coverage for Ne (blue squares) and Ar (red squares) on a  $(20,20)$  tube. For a better comparison, the energy per atom corresponding to the commensurate structure of coverage  $1/6$  was subtracted in both cases. (c) Same as in previous figures, but for Kr on top of a  $(20,20)$  tube using the C-Kr interaction of Ref. [9].

To improve the readability of the figure, we subtracted the energy corresponding to the commensurate  $\sqrt{3} \times \sqrt{3}$  structures ( $-348.9$  K for Ne and  $-1056.6$  K for Ar). The energy is lowest at a coverage of 0.265 for Ar and 0.403 for Ne. These values are different from those we measure at  $T \lesssim T_c$  (Fig. 3 of the Letter), suggesting that the monolayers observed in our experiments are not in the solid phase. These calculations were carried out with a  $(20,20)$  nanotube, but similar results were obtained with larger diameter nanotubes. We proceeded with finite  $T$  calculations where we considered the stability of various crystal structures with coverages similar to the values we measure at  $T \lesssim T_c$ . In all cases, these crystals melt below 5 K. The combination of our measurements and our calculations indicates that the monolayers observed experimentally are in the liquid phase.

The case of Kr is less conclusive. The experimental data with Kr are similar to that with Xe, suggesting that Kr monolayers might be commensurate solids. However, Fig. S8(c) shows that in the limit of zero temperature, the crystal is incommensurate. The data correspond to interaction parameters given in Ref. [9] (page 196). Similar results were obtained with more attractive potentials (those of Ref. [10] for C-Kr and Ref. [11] for Kr-Kr). The crystals, obtained with both interaction parameters, were calculated to melt at  $85 \pm 5$  K. In order to achieve a commensurate crystal, we had to artificially increase the anisotropic parameters by a factor of 4. We calculated that this crystal melts at  $55 \pm 3$  K, which is rather close to the measured value (Fig. S4). Further work is needed to clarify the case of Kr.

- 
- [1] C. Zhou, J. Kong, and H. Dai, *Physical Review Letters* **84**, 5604 (2000).
  - [2] V. Gouttenoire, T. Barois, S. Perisanu, J.-L. Leclercq, S. T. Purcell, P. Vincent, and A. Ayari, *Small* **6**, 1060 (2010).
  - [3] A. Eichler, M. del Álamo Ruiz, J. Plaza, and A. Bachtold, *Physical Review Letters* **109**, 025503 (2012).
  - [4] J. Chaste, M. Sledzinska, M. Zdrojek, J. Moser, and A. Bachtold, *Applied Physics Letters* **99**, 213502 (2011).
  - [5] L. Bruch and J. Venables, *Surface Science* **148**, 167 (1984).
  - [6] A. Cheng and M. L. Klein, *Langmuir* **8**, 2798 (1992).
  - [7] W. A. Steele, *The Journal of Physical Chemistry* **82**, 817 (1978).

- [8] M. L. Klein, S. O'Shea, and Y. Ozaki, *The Journal of Physical Chemistry* **88**, 1420 (1984).
- [9] L. W. Bruch, M. W. Cole, and E. Zaremba, Physical adsorption: forces and phenomena (Clarendon Press Oxford, 1997).
- [10] G. Vidali and M. W. Cole, *Phys. Rev. B* **29**, 6736 (1984).
- [11] H.-Y. Kim, M. W. Cole, M. Mbaye, and S. M. Gatica, *The Journal of Physical Chemistry A* **115**, 7249 (2011).
